# Supplementary material for: Block Mott insulating state induced by next-nearest neighbor hopping in the S = 3/2 zigzag chain BaCoTe2O7
Source: arXiv:2402.05389 source file (2024-05-06)
Supplement: Supplementary file 1 [file SuppMat.pdf]

## Supplementary Material

Ling-Fang Lin,<sup>1</sup> Yang Zhang,<sup>1</sup> Gonzalo Alvarez,<sup>2</sup> Adriana Moreo,<sup>1,3</sup> and Elbio Dagotto<sup>1,3</sup>

<sup>1</sup>*Department of Physics and Astronomy, University of Tennessee, Knoxville, Tennessee 37996, USA*

<sup>2</sup>*Computational Sciences and Engineering Division,*

*Oak Ridge National Laboratory, Oak Ridge, TN 37831, USA*

<sup>3</sup>*Materials Science and Technology Division, Oak Ridge National Laboratory, Oak Ridge, Tennessee 37831, USA*

(Dated: February 1, 2024)

## I. REPRODUCING THE DMRG RESULTS

Here, an example input file `chain_2.0.ain` is provided to reproduce the DMRG results presented in the main text. More details about DMRG++ software can be found at <https://github.com/g1257/dmrgpp> [1].

```
##Ainurl1.0;
TotalNumberOfSites=16;
NumberOfTerms=1;

DegreesOfFreedom=3;
GeometryKind="LongRange";
GeometryOptions="none";
integer GeometryMaxConnections=2;
matrix Connectors=[
[0,0,0,0.079,-0.027,-0.028,0.026,-0.007,-0.019,0,0,0,0,0,0,0,0,0,0,...],
[0,0,0,-0.027,-0.022,-0.009,0.007,-0.013,-0.038,0,0,0,0,0,0,0,0,0,0,...],
[0,0,0,0.028,0.009,0.003,0.019,-0.038,-0.124,0,0,0,0,0,0,0,0,0,0,...],
[0,0,0,0,0,0,0.079,0.027,-0.028,0.026,-0.007,-0.019,0,0,0,0,0,0,0,...],
[0,0,0,0,0,0,0.027,-0.022,-0.009,0.007,-0.013,-0.038,0,0,0,0,0,0,0,...],
[0,0,0,0,0,0,0.028,0.009,0.003,0.019,-0.038,-0.124,0,0,0,0,0,0,0,...],
[0,0,0,0,0,0,0,0,0.079,-0.027,-0.028,0.026,-0.007,-0.019,0,0,0,0,0,...],
[0,0,0,0,0,0,0,0,0,-0.027,-0.022,-0.009,0.007,-0.013,-0.038,0,0,0,0,...],
[0,0,0,0,0,0,0,0,0,0.028,0.009,0.003,0.019,-0.038,-0.124,0,0,0,0,...],
[0,0,0,0,0,0,0,0,0,0,0.079,0.027,-0.028,0.026,-0.007,-0.019,0,0,0,0,...],
[0,0,0,0,0,0,0,0,0,0,0,0.027,-0.022,-0.009,0.007,-0.013,-0.038,0,0,0,...],
[0,0,0,0,0,0,0,0,0,0,0,0,0.028,0.009,0.003,0.019,-0.038,-0.124,0,0,0,...],
[0,0,0,0,0,0,0,0,0,0,0,0,0,0.079,-0.027,-0.028,0.026,-0.007,-0.019,0,0,0,...],
[0,0,0,0,0,0,0,0,0,0,0,0,0,0,0.027,-0.022,-0.009,0.007,-0.013,-0.038,0,0,0,...],
[0,0,0,0,0,0,0,0,0,0,0,0,0,0,0,0.028,0.009,0.003,0.019,-0.038,-0.124,0,0,0,...],
[0,0,0,0,0,0,0,0,0,0,0,0,0,0,0,0,0.079,-0.027,-0.028,0.026,-0.007,-0.019,0,0,0,...],
[... ,0,0.027,-0.022,-0.009,0.007,-0.013,-0.038,0,0,0,0,0,0,0,0,0,0,0,0],
[... ,0,0.028,0.009,0.003,0.019,-0.038,-0.124,0,0,0,0,0,0,0,0,0,0,0,0],
[... ,0,0,0.079,-0.027,-0.028,0.026,-0.007,-0.019,0,0,0,0,0,0,0,0,0,0,0],
[... ,0,0,0,-0.027,-0.022,-0.009,0.007,-0.013,-0.038,0,0,0,0,0,0,0,0,0,0,0],
[... ,0,0,0,0.028,0.009,0.003,0.019,-0.038,-0.124,0,0,0,0,0,0,0,0,0,0,0],
[... ,0,0,0,0,0,0.079,0.027,-0.028,0.026,-0.007,-0.019,0,0,0,0,0,0,0,0,0],
[... ,0,0,0,0,0,0,0.027,-0.022,-0.009,0.007,-0.013,-0.038,0,0,0,0,0,0,0,0],
[... ,0,0,0,0,0,0,0,0.028,0.009,0.003,0.019,-0.038,-0.124,0,0,0,0,0,0,0],
[... ,0,0,0,0,0,0,0,0,0.079,-0.027,-0.028,0.026,-0.007,-0.019,0,0,0,0,0,0],
[... ,0,0,0,0,0,0,0,0,0,-0.027,-0.022,-0.009,0.007,-0.013,-0.038,0,0,0,0,0],
[... ,0,0,0,0,0,0,0,0,0,0.028,0.009,0.003,0.019,-0.038,-0.124,0,0,0,0,0],
```

```
[... ,0,0,0,0,0,0,0,0,0,0,0,0,0,0,0,0,0.079,0.027,-0.028,0.026,-0.007,-0.019,0,0,0,0,0,0],
[... ,0,0,0,0,0,0,0,0,0,0,0,0,0,0,0,0,0.027,-0.022,-0.009,0.007,-0.013,-0.038,0,0,0,0,0,0],
[... ,0,0,0,0,0,0,0,0,0,0,0,0,0,0,0,0,0.028,0.009,0.003,0.019,-0.038,-0.124,0,0,0,0,0,0],
[... ,0,0,0,0,0,0,0,0,0,0,0,0,0,0,0,0,0.079,-0.027,-0.028,0.026,-0.007,-0.019,0,0,0,0,0],
[... ,0,0,0,0,0,0,0,0,0,0,0,0,0,0,0,0,-0.027,-0.022,-0.009,0.007,-0.013,-0.038,0,0,0,0,0],
[... ,0,0,0,0,0,0,0,0,0,0,0,0,0,0,0,0,0.028,0.009,0.003,0.019,-0.038,-0.124,0,0,0,0,0],
[... ,0,0,0,0,0,0,0,0,0,0,0,0,0,0,0,0,0.079,0.027,-0.028,0.026,-0.007,-0.019],
[... ,0,0,0,0,0,0,0,0,0,0,0,0,0,0,0,0,0.027,-0.022,-0.009,0.007,-0.013,-0.038],
[... ,0,0,0,0,0,0,0,0,0,0,0,0,0,0,0,0,0.028,0.009,0.003,0.019,-0.038,-0.124],
[... ,0,0,0,0,0,0,0,0,0,0,0,0,0,0,0,0,0.079,-0.027,-0.028],
[... ,0,0,0,0,0,0,0,0,0,0,0,0,0,0,0,0,-0.027,-0.022,-0.009],
[... ,0,0,0,0,0,0,0,0,0,0,0,0,0,0,0,0,0.028,0.009,0.003],
[... ,0,0,0,0,0,0,0,0,0,0,0,0,0,0,0,0,0,0,0,0,0,0,0,0,0,0],
[... ,0,0,0,0,0,0,0,0,0,0,0,0,0,0,0,0,0,0,0,0,0,0,0,0,0,0],
[... ,0,0,0,0,0,0,0,0,0,0,0,0,0,0,0,0,0,0,0,0,0,0,0,0,0,0]];
```

```
#There are 4 values of U
#Taken from ParametersModelFeAs.h
#std::cout<<"U[0]="<<hubbardU[0]<<" U
n";
#std::cout<<"U[1]="<<hubbardU[1]<<" U'-J/2
n";
#std::cout<<"U[2]="<<hubbardU[2]<<" -2J for S+S- + S-S+ term
n";
#std::cout<<"U[3]="<<hubbardU[3]<<" -J
n";
hubbardU=[2.0, .75000, -1, -0.5];
```

```
potentialV=[
-0.072, -0.072, -0.072, -0.072, -0.072, -0.072, -0.072, -0.072, -0.072, -0.072, -0.072, -0.072, -0.072,
-0.072, -0.072, -0.072,
-0.397, -0.397, -0.397, -0.397, -0.397, -0.397, -0.397, -0.397, -0.397, -0.397, -0.397, -0.397, -0.397,
-0.397, -0.397, -0.397,
0.477, 0.477, 0.477, 0.477, 0.477, 0.477, 0.477, 0.477, 0.477, 0.477, 0.477, 0.477, 0.477, 0.477,
0.477, 0.477,
-0.072, -0.072, -0.072, -0.072, -0.072, -0.072, -0.072, -0.072, -0.072, -0.072, -0.072, -0.072, -0.072,
-0.072, -0.072, -0.072,
-0.397, -0.397, -0.397, -0.397, -0.397, -0.397, -0.397, -0.397, -0.397, -0.397, -0.397, -0.397, -0.397,
-0.397, -0.397, -0.397,
0.477, 0.477, 0.477, 0.477, 0.477, 0.477, 0.477, 0.477, 0.477, 0.477, 0.477, 0.477, 0.477, 0.477,
0.477, 0.477];
Model="FeAsBasedSc";
FeAsMode="INT_PAPER33";
Orbitals=3;
SolverOptions="none";
Version="version";
OutputFile="data0";
InfiniteLoopKeptStates=200;
FiniteLoops=[
[7, 400, 0],
[-14, 400, 0], [14, 400, 0],
[-14, 600, 0], [14, 600, 0],
[-14, 700, 0], [14, 700, 0],
[-14, 800, 0], [14, 800, 0],
[-14, 900, 0], [14, 900, 0],
[-14, 900, 0], [14, 900, 0],
[-14, 1000, 0], [14, 1000, 0],
```

```

[-14, 1000, 0], [14, 1000, 0],
[-14, 1100, 0], [14, 1100, 0],
[-14, 1100, 0], [14, 1100, 0],
[-14, 1200, 0], [14, 1200, 0],
[-14, 1200, 0], [14, 1200, 1]];
TargetElectronsUp=24;
TargetElectronsDown=24;
Threads=4;
string DefineOperators=na:n?0+n?3,nb:n?1+n?4,nc:n?2+n?5,nt:na+nb+nc;

```

Note that `matrix Connectors` should be a 48 matrix, which is too large to show in a whole piece so that we discard some zeros here.

Here are some commands for calculating ground state and measuring observables.

```

dmrg -f chain_2.0.ain -p 10 >dmrg.dat
observe -f chain_2.0.ain ss >ss.dat
observe -f chain_2.0.ain "<gs|na|gs>,<gs|nb|gs>,<gs|nc|gs>" >nn.dat
observe -f chain_2.0.ain "<gs|na*na|gs>" >>nasq.dat
observe -f chain_2.0.ain "<gs|nb*nb|gs>" >>nbsq.dat
observe -f chain_2.0.ain "<gs|nc*nc|gs>" >>ncsq.dat
observe -f chain_2.0.ain "<gs|nt*nt|gs>" >>ntsqsq.dat
observe -f chain_2.0.ain "<gs|nt|gs>" >>nt.dat
observe -f chain_2.0.ain "<gs|na;na|gs>,<gs|nb;nb|gs>,<gs|nc;nc|gs>,<gs|nt;nt|gs>" > nn1.dat

```

- 
- [1] G. Alvarez, The density matrix renormalization group for strongly correlated electron systems: A generic implementation, *Comput. Phys. Commun.* **180**, 1572 (2009).
